# Supplementary material for: Lazy Contracts: Alleviating High Gas Costs by Secure and Trustless Off-chain Execution of Smart Contracts
Source: arXiv:2309.11317 source file (2023-09-20)
Supplement: Supplementary file 1 [file appendix1.tex]

%!TEX program = xelatex
%!TEX root = ./thesis.tex
\chapter{Appendix 1}
